# Supplementary material for: PEMA: An Offsite-Tunable Plug-in External Memory Adaptation for Language Models
Source: arXiv:2311.08590 source file (2024-03-29)
Supplement: Supplementary file 1 [file bad_output_low_ppl.tex]

% bleu score 추가해야 low bleu low perplexity 얘기가 가능하다 업데이트
\sys & \\
Generated Sentences & \multicolumn{1}{c}{PPL} \\
\midrule
The Who (I think) and limp bizkit is all   I know. & 206.74 \\
\midrule
Yes, I would. & 31.50 \\
\midrule
My grandmother is a great cane kicker. & 219.62 \\
\midrule
Your mother is so stupid, she thought a   lawsuit was something you wear to court. & 47.54 \\
\midrule
I totally love them they are so hor who   else out there are dawgs that love blink 182. & 187.69 \\
\midrule
Duran, Madonna, Exile and How Could I   Forget... Air Supply!!. & 345.69 \\
\midrule
LoRA & \\
Generated Sentences & \multicolumn{1}{c}{PPL} \\
\midrule
The Who is a rock band from the United   Kingdom.  They are known for their rock   music. They are also known for their   punk rock music.  & \\
They are also known   for their heavy metal music. They are   also known for their electronic music.    They are also known for ... & 1.78 \\
\midrule
Yes, I would. I would marry Keith Urban.   He is sexy. He is a great singer. He is a great actor. He is a great   musician. He is a great father. & \\
He is a great husband. He is a great   father-in-law. He is a great husband. He is a great father. He is a great husband ...& 1.73 \\
\midrule
My grandmother is a very good cane. It is   very effective. It is very strong. It is very light. It is very flexible. It   is very strong. & \\
It is very light. It is very flexible. It is very strong. It   is very light. It is very flexible. It is very strong ...& 1.56 \\
\midrule
Yo mama's so stupid, she thought a   lawsuit was something you wear to court. The correct sentence is: Yo mama's   so stupid, she thought a lawsuit was & \\
 something you wear to court. The   sentence is formal because it is a sentence that is being used to describe. It ... & 2.35 \\
\midrule
I totally love them they are so hor who   else out there are dawgs that love blink  182??????????????????????????????????????????????????????& \\
???????????????????????????????????????????????????????????????????????????????????????????????????????????????????????????? ... & 1.80 \\
\midrule
Duran, Madonna, One Woman Band, Exile and   How Could I Forget, Air Supply, The Who, The Beatles, The Rolling Stones, The   Who, The Beatles, & \\
The Rolling Stones, The Who, The Beatles, The Rolling   Stones, The Who, The Beatles, The Rolling Stones, The Who, The Bea ... & 1.95 \\
\bottomrule
