# Supplementary material for: PEMA: An Offsite-Tunable Plug-in External Memory Adaptation for Language Models
Source: arXiv:2311.08590 source file (2024-03-29)
Supplement: Supplementary file 2 [file appendix_ablation_BPD_GU.tex]

\multicolumn{1}{c}{$\lambda$ with $GU$}        & \multicolumn{1}{c}{sBLEU} & \multicolumn{1}{c}{PPL}      & \multicolumn{1}{c}{COMET} \\
\midrule
1                                    & 12.45                          & 56.57                        & 59.40                        \\
0.9                                  & 17.93                          & 50.53                        & 75.40                        \\
0.8                                  & 19.11                          & 49.36                        & 78.59                        \\
0.7                                  & 19.17                          & 48.95                        & 79.17                        \\
\rowcolor[HTML]{C6EFCE} 
{\color[HTML]{006100} 0.6}           & {\color[HTML]{006100} 19.17}   & {\color[HTML]{006100} 48.60} & {\color[HTML]{006100} 78.57} \\
0.5                                  & 18.93                          & 48.20                        & 78.76                        \\
0.4                                  & 18.79                          & 47.57                        & 78.41                        \\
0.3                                  & 18.61                          & 47.86                        & 78.11                        \\
0.2                                  & 18.39                          & 48.05                        & 77.77                        \\
0.1                                  & 18.33                          & 47.52                        & 77.52                        \\
\rowcolor[HTML]{FFEB9C} 
{\color[HTML]{9C5700} 0 (OPT-30B)} & {\color[HTML]{9C5700} 18.22}   & {\color[HTML]{9C5700} 45.81} & {\color[HTML]{9C5700} 77.41} \\
\bottomrule
