# Supplementary material for: PEMA: An Offsite-Tunable Plug-in External Memory Adaptation for Language Models
Source: arXiv:2311.08590 source file (2024-03-29)
Supplement: Supplementary file 3 [file appendix_ablation_BPD_GU_RCT.tex]

\multicolumn{1}{c}{$\lambda$ with $GU$}        & \multicolumn{1}{c}{sBLEU}    & \multicolumn{1}{c}{PPL}      & \multicolumn{1}{c}{COMET}    \\
\midrule
1                                    & 12.55                        & 52.28                        & 61.10                        \\
0.9                                  & 18.50                        & 47.45                        & 76.42                        \\
0.8                                  & 19.12                        & 46.61                        & 78.60                        \\
\rowcolor[HTML]{C6EFCE} 
{\color[HTML]{006100} 0.7}           & {\color[HTML]{006100} 19.22} & {\color[HTML]{006100} 46.62} & {\color[HTML]{006100} 79.21} \\
0.6                                  & 19.11                        & 46.18                        & 78.90                        \\
0.5                                  & 18.95                        & 46.12                        & 78.69                        \\
0.4                                  & 18.82                        & 46.03                        & 78.48                        \\
0.3                                  & 18.57                        & 45.85                        & 78.08                        \\
0.2                                  & 18.37                        & 45.89                        & 77.73                        \\
0.1                                  & 18.28                        & 45.84                        & 77.46                        \\
\rowcolor[HTML]{FFEB9C} 
{\color[HTML]{9C5700} 0 (OPT-30B)} & {\color[HTML]{9C5700} 18.22} & {\color[HTML]{9C5700} 45.81} & {\color[HTML]{9C5700} 77.41}\\
\bottomrule
