# Supplementary material for: PEMA: An Offsite-Tunable Plug-in External Memory Adaptation for Language Models
Source: arXiv:2311.08590 source file (2024-03-29)
Supplement: Supplementary file 5 [file comparison_with_lora_same_parameters.tex]

WMT22 (EN$\rightarrow$DE)& \multicolumn{1}{c}{sBLEU} & \multicolumn{1}{c}{PPL} & \multicolumn{1}{c}{COMET} \\
\midrule
OPT-IML-MAX-30B (LoRA) & 16.03& \textbf{46.97}& 74.65 \\
OPT-IML-MAX-30B (PEMA w/o rct) & \textbf{19.17}& 48.60 & \textbf{79.12} \\
\midrule
GYAFC (Family \& Relationships)& \multicolumn{1}{c}{sBLEU} & \multicolumn{1}{c}{PPL} & \multicolumn{1}{c}{FormImp} \\
\midrule
OPT-IML-MAX-30B (LoRA) & 61.39 & \textbf{22.00} & \textbf{73.10}\\
OPT-IML-MAX-30B (PEMA w/o rct) & \textbf{70.29}& 23.38 & 51.24 \\
\midrule
GYAFC (Entertainment \& Music)& \multicolumn{1}{c}{sBLEU} & \multicolumn{1}{c}{PPL} & \multicolumn{1}{c}{FormImp}  \\
\midrule
OPT-IML-MAX-30B (LoRA) & 59.76 & \textbf{23.97}& \textbf{68.29}\\
OPT-IML-MAX-30B (PEMA w/o rct) & \textbf{64.82}& 26.32 & 42.61\\
\bottomrule
