# Supplementary material for: PEMA: An Offsite-Tunable Plug-in External Memory Adaptation for Language Models
Source: arXiv:2311.08590 source file (2024-03-29)
Supplement: Supplementary file 6 [file model_comparison_rank.tex]

Model & \multicolumn{3}{c}{WMT22 (EN$\rightarrow$DE)} & \multicolumn{3}{c}{GYAFC (F\&R)} & \multicolumn{3}{c}{GYAFC (E\&M)}\\
& \multicolumn{1}{c}{sBLEU} & \multicolumn{1}{c}{PPL} & \multicolumn{1}{c}{COMET} & \multicolumn{1}{c}{sBLEU} & \multicolumn{1}{c}{PPL} & \multicolumn{1}{c}{FormImp} & \multicolumn{1}{c}{sBLEU} & \multicolumn{1}{c}{PPL} & \multicolumn{1}{c}{FormImp} \\
\midrule
OPT-1.3B (LoRA${}_{r=8}$) & 3.25& 66.16 & 40.50 & 23.13 & \textbf{18.82} & {\underline{45.68}} & 18.41 & {\textbf{19.68}} & {\underline{46.00}} \\
OPT-1.3B (LoRA${}_{r=512}$) & 4.28& 61.25& 39.32 & 20.98 & {\underline{19.07}} & \textbf{45.71}& 15.57 & \underline{19.71}& \textbf{46.32}\\
OPT-1.3B (PEMA${}_{r=8}$) & {\underline{11.75}} & {\underline{44.73}} & {\underline{61.50}} & {\underline{56.29}} & 21.41 & 36.27 & {\underline{54.22}} & 23.42 & 35.52 \\
OPT-1.3B (PEMA${}_{r=512}$) & \textbf{12.87}& \textbf{42.62}& \textbf{64.16}& \textbf{64.82}& 23.15& 41.90 & \textbf{61.24}& 24.28 & 36.28 \\
\midrule
LLaMA-7B (LoRA${}_{r=8}$) & 10.92 & 52.01 & 66.88 & 14.80 & \textbf{17.85}& \textbf{88.43}& 12.69 & \textbf{19.66} & \textbf{89.70}\\
LLaMA-7B (LoRA${}_{r=512}$) & {\underline{11.46}} & \underline{51.36} & {\underline{67.48}} & {\underline{52.67}} & \underline{22.42} & 72.23 & \underline{52.15} & \underline{24.74} & {\underline{71.28}} \\
LLaMA-7B (PEMA${}_{r=8}$) & 3.88& \textbf{45.48} & 48.44 & 48.88 & 26.69 & {\underline{80.21}} & 45.73 & 32.03 & 70.85 \\
LLaMA-7B (PEMA${}_{r=512}$) & \textbf{14.50}& 54.26 & \textbf{70.31}& \textbf{63.99}& 23.19 & 61.40 & \textbf{60.88} & 26.00 & 60.94 \\
\midrule
OPT-30B (LoRA${}_{r=8}$)& 16.05 & 47.66 & 74.01 & 61.28 & {\underline{21.99}} & \textbf{73.33}& 59.48 & {\underline{24.01}} & \textbf{68.35}\\
OPT-30B (LoRA${}_{r=512}$)& 16.03& \underline{46.97}& 74.65 & 61.39 & 22.00 & {\underline{73.10}} & 59.76 & \textbf{23.97}& {\underline{68.29}} \\
OPT-30B (PEMA${}_{r=8}$)& {\underline{18.33}} & 47.40 & {\underline{77.75}} & {\underline{62.87}} & \textbf{21.75} & 46.05 & {\underline{60.12}} & 24.10 & 38.92 \\
OPT-30B (PEMA${}_{r=512}$)& \textbf{19.22}& {\textbf{46.62}} & \textbf{79.21}& \textbf{70.84}& 22.04& 52.35 & \textbf{65.43}& 25.53 & 44.63\\
\bottomrule
