# Supplementary material for: PEMA: An Offsite-Tunable Plug-in External Memory Adaptation for Language Models
Source: arXiv:2311.08590 source file (2024-03-29)
Supplement: Supplementary file 9 [file appendix_ablation_BPD_selection.tex]

\multicolumn{1}{c}{Lambda}           & \multicolumn{1}{c}{sBLEU} & \multicolumn{1}{c}{PPL}      & \multicolumn{1}{c}{COMET} \\
\midrule
1                                    & 0.47                           & 67.75                         & 22.00                        \\
0.9                                  & 3.01                           & 59.11                         & 32.68                        \\
0.8                                  & 4.86                           & 59.09                        & 56.11                        \\
0.7                                  & 5.10                           & 59.54                        & 65.82                        \\
0.6                                  & 5.20                           & 59.08                        & 69.10                        \\
0.5                                  & 7.77                           & 54.50                        & 72.58                        \\
\rowcolor[HTML]{C6EFCE} 
{\color[HTML]{006100} 0.4}           & {\color[HTML]{006100} 18.74}   & {\color[HTML]{006100} 48.05} & {\color[HTML]{006100} 77.76} \\
0.3                                  & 18.58                          & 47.82                        & 77.80                        \\
0.2                                  & 18.39                          & 47.63                        & 77.71                        \\
0.1                                  & 18.32                          & 47.56                        & 77.47                        \\
\rowcolor[HTML]{FFEB9C} 
{\color[HTML]{9C5700} 0 (naïve-opt)} & {\color[HTML]{9C5700} 18.22}   & {\color[HTML]{9C5700} 45.81} & {\color[HTML]{9C5700} 77.41} \\
\bottomrule
